# Supplementary material for: Jade: A Differentiable Physics Engine for Articulated Rigid Bodies with Intersection-Free Frictional Contact
Source: arXiv:2309.04710 source file (2023-09-09)
Supplement: Supplementary file 1 [file appendix.tex]

\section{Dantzig's Function Details}

The calculation details of functions \textsc{SolveDf}, \textsc{MaxStep} and \textsc{TransitSet} are summarized in Alg.\ref{alg:function}. And the calculation details of functions \textsc{SolveDfFriction}, \textsc{MaxStepFriction} and \textsc{TransitSetFriction} are summarized in Alg.\ref{alg:function_friction_1}\ref{alg:function_friction_2}\ref{alg:function_friction_3}. In Alg.\ref{alg:function_friction_2}, we compare the original algorithm (in red) and our modification (in blue).

\begin{algorithm}[ht]
\caption{Dantzig’s Algorithm (no friction)}
\label{alg:function}
\begin{algorithmic}[1] 

\State \textbf{given} matrix $\M$, vector $\vel$, set $\cs, \ct$ and index $i$
\State $\M_{\cs\ct}$ is the matrix of $\M$'s $\cs$ rows and $\ct$ cols
\State $\M_{\cs i}$ is the vector of $\M$'s $\cs$ rows and $i$th col
\State $\M_{* i}$ is the vector of $\M$'s $i$th col
\State $\vel_\cs$ is the vector of $\vel$'s $\cs$ components

\State 

\Function{SolveDf}{$k$}
    \State $\Delta \f \gets \0$
    \State $\Delta f_k \gets 1$
    \State $\Delta f_\cc \gets - \A_{\cc\cc}^{-1}\A_{\cc k}$
    \State \textbf{return} $\Delta \f$
\EndFunction

\State

\Function{MaxStep}{$k, \Delta \f$}
    \State $\s \gets \infty$
    \For{$i \in \cc$}
        \If{$\Delta f_i < 0$}
            \State $s_i \gets - f_i / \Delta f_i$
        \EndIf
    \EndFor
    \For{$i \in \cn$}
        \If{$\Delta a_i < 0$}
            \State $s_i \gets - a_i / \Delta a_i$
        \EndIf
    \EndFor
    \State $s_k \gets - a_k / \Delta a_k$
    \State \textbf{return} $\s$
\EndFunction

\State

\Function{TransitSet}{$j$}
    \If{$j \in \cc$}
        \State $\cc \gets \cc - \{j\}$
        \State $\cn \gets \cn \cup \{j\}$
    \ElsIf{$j \in \cn$}
        \State $\cn \gets \cn - \{j\}$
        \State $\cc \gets \cc \cup \{j\}$
    \Else
        \State $\cc \gets \cc \cup \{j\}$
    \EndIf
\EndFunction

\end{algorithmic}
\end{algorithm}

%%%%%
\begin{algorithm}[ht]
\caption{Dantzig’s Algorithm (static friction)}
\label{alg:function_friction_1}
\begin{algorithmic}[1] 

\State \textbf{given} an friction index $i$
\State $N(i)$ denotes the index of corresponding normal force
\State $\mu(i)$ denotes the friction coefficient

\State 

\Function{SolveDfFriction}{$k$}
    \State $\Delta \f \gets \0$
    \State $\A^{\prime} \gets \A$ \Comment{make a copy of $\A$}
    \For{$i \in \cnh$}
        \State $\A^\prime_{*N(i)} \gets \A^\prime_{*N(i)} + \mu(i) \A^\prime_{*i}$ 
    \EndFor
    \For{$i \in \cnl$}
        \State $\A^\prime_{*N(i)} \gets \A^\prime_{*N(i)} - \mu(i) \A^\prime_{*i}$ 
    \EndFor
    \State
    \State \textbf{let} $\ccl = \cc \cup \ccf$
    \If{$a_k < 0$}
        \State $\Delta f_k \gets 1$
        \State $\Delta f_\ccl \gets - \A^{\prime-1}_{\ccl\ccl}\A_{\ccl k}$
    \ElsIf{$a_k > 0$}
        \State $\Delta f_k \gets -1$
        \State $\Delta f_\ccl \gets \A^{\prime-1}_{\ccl\ccl}\A_{\ccl k}$
    \EndIf
    \For{$i \in \cnh$}
        \State $\Delta f_i \gets \mu(i) \Delta f_{N(i)}$
    \EndFor
    \For{$i \in \cnl$}
        \State $\Delta f_i \gets - \mu(i) \Delta f_{N(i)}$ 
    \EndFor
    \State
    \State \textbf{return} $\Delta \f$
\EndFunction

\end{algorithmic}
\end{algorithm}

\begin{algorithm}[ht]
\caption{Dantzig’s Algorithm (static friction)}
\label{alg:function_friction_2}
\begin{algorithmic}[1] 

\Function{MaxStepFriction}{$k, \Delta \f$}
    \State $\s \gets \infty$
    \For{$i \in \cc$}
        \If{$\Delta f_i < 0$}
            \State $s_i \gets - f_i / \Delta f_i$
        \EndIf
    \EndFor
    \For{$i \in \ccf$}
        \If{$\Delta f_i > 0$}
            \color{red}
            \State $s_i \gets (\mu(i) \Delta f_{N(i)} - f_i) / \Delta f_i$
            \color{blue}
            \State $s_i \gets (\mu(i) \Delta f_{N(i)} - f_i) / (\Delta f_i - \mu(i) \Delta f_{N(i)})$
            \color{black}
        \ElsIf{$\Delta f_i < 0$}
            \color{red}
            \State $s_i \gets (-\mu(i) \Delta f_{N(i)} - f_i) / \Delta f_i$
            \color{blue}
            \State $s_i \gets (- \mu(i) \Delta f_{N(i)} - f_i) / (\Delta f_i + \mu(i) \Delta f_{N(i)})$
            \color{black}
        \EndIf
    \EndFor
    \For{$i \in \cn \cup \cnh \cup \cnl$}
        \If{$\Delta a_i > 0$}
            \State $s_i \gets - a_i / \Delta a_i$
        \EndIf
    \EndFor
    \State
    \State \textbf{let} $s_a = - a_k / \Delta a_k$
    \If{$\Delta f_k > 0$}
        \color{red}
        \State \textbf{let} $s_f = (\mu(k) \Delta f_{N(k)} - f_k) / \Delta f_k$
        \color{blue}
        \State \textbf{let} $s_f = (\mu(k) \Delta f_{N(k)} - f_k) / (\Delta f_k - \mu(k) \Delta f_{N(k)})$
        \color{black}
    \ElsIf{$\Delta f_i < 0$}
        \color{red}
        \State \textbf{let} $s_f = (- \mu(k) \Delta f_{N(k)} - f_k) / \Delta f_k$
        \color{blue}
        \State \textbf{let} $s_f = (- \mu(k) \Delta f_{N(k)} - f_k) / (\Delta f_k + \mu(k) \Delta f_{N(k)})$
        \color{black}
    \EndIf
    \State $s_k \gets \min(s_a, s_f)$
    \State
    \State \textbf{return} $\s$
\EndFunction

\end{algorithmic}
\end{algorithm}

\begin{algorithm}[ht]
\caption{Dantzig’s Algorithm (static friction)}
\label{alg:function_friction_3}
\begin{algorithmic} 

\Function{TransitSetFriction}{$j$}
    \If{$j \in \cc$}
        \State $\cc \gets \cc - \{j\}$
        \State $\cn \gets \cn \cup \{j\}$
    \ElsIf{$j \in \cn$}
        \State $\cn \gets \cn - \{j\}$
        \State $\cc \gets \cc \cup \{j\}$
    \ElsIf{$j \in \ccf$}
        \State $\ccf \gets \ccf - \{j\}$
        \If{$\Delta f_i > 0$}
            \State $\cnh \gets \cnh \cup \{j\}$
        \ElsIf{$\Delta f_i < 0$}
            \State $\cnl \gets \cnh \cup \{j\}$
        \EndIf
    \ElsIf{$j \in \cnh$}
        \State $\cnh \gets \cnh - \{j\}$
        \State $\ccf \gets \ccf \cup \{j\}$
    \ElsIf{$j \in \cnl$}
        \State $\cnl \gets \cnl - \{j\}$
        \State $\ccf \gets \ccf \cup \{j\}$
    \Else
        \If{$f_k = \mu(k) \Delta f_{N(k)}$}
            \State $\cnh \gets \cnh \cup \{k\}$
        \ElsIf{$f_k = - \mu(k) \Delta f_{N(k)}$}
            \State $\cnl \gets \cnl \cup \{k\}$
        \Else
            \State $\ccf \gets \ccf \cup \{k\}$
        \EndIf
    \EndIf
\EndFunction

\end{algorithmic}
\end{algorithm}

% \section{Time Cost Analysis}

\clearpage

\section{End-to-end Backward Differentiation}

According to Eq.\ref{eq:1}, the backward differentiation formula of the whole forward dynamics in one timestep with several collisions is recursive and depends on the number of collisions. To have impression of it, consider one timestep with 2 collisions. Let $(\J)_c$ denote the Jacobian of collision point’s normal component, $[\q^-_3, \dq^-_3]$ denote $[\q_{t+1}, \dq_{t+1}]$ and $[\q^+_0, \dq^+_0]$ denote $[\q_{t}, \dq_{t}]$. The differentiation formula of Eq.\ref{eq:1} is as below:

Differentiate $[\q^-_3, \dq^-_3] = P(\q^+_2, \dq^+_2, \m, \tf, \dt - \dt_0 - \dt_1)$:
\begin{align}
    &\left \{
    \begin{aligned}
    \frac{\partial \q^-_3}{\partial \q^+_2} =& \I  ,\; \frac{\partial \q^-_3}{\partial \dq^+_2} = \dt_2 \I \\
    \frac{\partial \q^-_3}{\partial \dt_0} =& -\dq^+_2 ,\; \frac{\partial \q^-_3}{\partial \dt_1} = -\dq^+_2
    \end{aligned}
    \right. \\
    &\left \{
    \begin{aligned}
    \frac{\partial \dq^-_3}{\partial \q^+_2} =& \frac{\partial (\M^+_2)^{-1}}{\partial \q^+_2} (\dt_2(\tf - \corio^+_2) + (\J^+_2)^T\f^+_2) \\
    +& (\M^+_2)^{-1}(-\dt_2 \frac{\partial \corio^+_2}{\partial \q^+_2} + \frac{\partial (\J^+_2)^T}{\partial \q^+_2}\f^+_2) + (\J^+_2)^T\frac{\partial \f^+_2}{\partial \q^+_2}  \\
    \frac{\partial \dq^-_3}{\partial \dq^+_2} =& \I + (\M^+_2)^{-1}(-\dt_2 \frac{\partial \corio^+_2}{\partial \dq^+_2} + (\J^+_2)^T\frac{\partial \f^+_2}{\partial \dq^+_2}) \\
    \frac{\partial \dq^-_3}{\partial \tf} =& (\M^+_2)^{-1}(\dt_2 \I + (\J^+_2)^T \frac{\partial \f^+_2}{\partial \tf}) \\
    \frac{\partial \dq^-_3}{\partial \m} =& \frac{\partial (\M^+_2)^{-1}}{\partial \m} (\dt_2(\tf - \corio^+_2) + (\J^+_2)^T\f^+_2) \\ 
    +& (\M^+_2)^{-1}(-\dt_2 \frac{\partial \corio^+_2}{\partial \m} + (\J^+_2)^T \frac{\partial \f^+_2}{\partial \m}) \\
    \frac{\partial \dq^-_3}{\partial \dt_0} =& -(\M^+_2)^{-1} ((\tf - \corio^+_2) + (\J^+_2)^T\f^+_2 / \dt_2) \\
    \frac{\partial \dq^-_3}{\partial \dt_1} =& -(\M^+_2)^{-1} ((\tf - \corio^+_2) + (\J^+_2)^T\f^+_2 / \dt_2)
    \end{aligned}
    \right.
\end{align}

Differentiate $[\q^+_2, \dq^+_2] = C(\q^-_2, \dq^-_2, \m)$:
\begin{equation}
    \left \{
    \begin{aligned}
    \frac{\partial \q^+_2}{\partial \q^-_2} =& \I \\
    \frac{\partial \dq^+_2}{\partial \q^-_2} =& \frac{\partial (\M^-_2)^{-1}}{\partial \q^-_2} (\J^-_2)^T\f^-_2 \\
    +& (\M^+_2)^{-1}\frac{\partial (\J^-_2)^T}{\partial \q^-_2}\f^-_2 + (\J^-_2)^T\frac{\partial \f^-_2}{\partial \q^-_2}  \\
    \frac{\partial \dq^+_2}{\partial \dq^-_2} =& \I + (\M^-_2)^{-1}(\J^-_2)^T\frac{\partial \f^-_2}{\partial \dq^-_2} \\
    \frac{\partial \dq^+_2}{\partial \m} =& \frac{\partial (\M^-_2)^{-1}}{\partial \m} (\J^-_2)^T\f^-_2 + (\M^-_2)^{-1}(\J^-_2)^T \frac{\partial \f^-_2}{\partial \m}
    \end{aligned}
    \right. 
\end{equation}

Differentiate $[\q^-_2, \dq^-_2] = P(\q^+_1, \dq^+_1, \m, \tf, \dt_1)$:
\begin{align}
    &\left \{
    \begin{aligned}
    \frac{\partial \q^-_2}{\partial \q^+_1} =& \I  ,\; \frac{\partial \q^-_2}{\partial \dq^+_1} = \dt_1 \I \\
    \frac{\partial \q^-_2}{\partial \dt_1} =& \dq^+_1
    \end{aligned}
    \right. \\
    &\left \{
    \begin{aligned}
    \frac{\partial \dq^-_2}{\partial \q^+_1} =& \frac{\partial (\M^+_1)^{-1}}{\partial \q^+_1} (\dt_1(\tf - \corio^+_1) + (\J^+_1)^T\f^+_1) \\
    +& (\M^+_1)^{-1}(-\dt_1 \frac{\partial \corio^+_1}{\partial \q^+_1} + \frac{\partial (\J^+_1)^T}{\partial \q^+_1}\f^+_1) + (\J^+_1)^T\frac{\partial \f^+_1}{\partial \q^+_1}  \\
    \frac{\partial \dq^-_2}{\partial \dq^+_1} =& \I + (\M^+_1)^{-1}(-\dt_1 \frac{\partial \corio^+_1}{\partial \dq^+_1} + (\J^+_1)^T\frac{\partial \f^+_1}{\partial \dq^+_1}) \\
    \frac{\partial \dq^-_2}{\partial \tf} =& (\M^+_1)^{-1}(\dt_1 \I + (\J^+_1)^T \frac{\partial \f^+_1}{\partial \tf}) \\
    \frac{\partial \dq^-_2}{\partial \m} =& \frac{\partial (\M^+_1)^{-1}}{\partial \m} (\dt_1(\tf - \corio^+_1) + (\J^+_1)^T\f^+_1) \\ 
    +& (\M^+_1)^{-1}(-\dt_1 \frac{\partial \corio^+_1}{\partial \m} + (\J^+_1)^T \frac{\partial \f^+_1}{\partial \m}) \\
    \frac{\partial \dq^-_2}{\partial \dt_1} =& (\M^+_1)^{-1} ((\tf - \corio^+_1) + (\J^+_1)^T\f^+_1 / \dt_1)
    \end{aligned}
    \right. 
\end{align}

Differentiate $[\q^+_1, \dq^+_1] = C(\q^-_1, \dq^-_1, \m)$:
\begin{equation}
    \left \{
    \begin{aligned}
    \frac{\partial \q^+_1}{\partial \q^-_1} =& \I \\
    \frac{\partial \dq^+_1}{\partial \q^-_1} =& \frac{\partial (\M^-_1)^{-1}}{\partial \q^-_1} (\J^-_1)^T\f^-_1 \\
    +& (\M^+_1)^{-1}\frac{\partial (\J^-_1)^T}{\partial \q^-_1}\f^-_1 + (\J^-_1)^T\frac{\partial \f^-_1}{\partial \q^-_1}  \\
    \frac{\partial \dq^+_1}{\partial \dq^-_1} =& \I + (\M^-_1)^{-1}(\J^-_1)^T\frac{\partial \f^-_1}{\partial \dq^-_1} \\
    \frac{\partial \dq^+_1}{\partial \m} =& \frac{\partial (\M^-_1)^{-1}}{\partial \m} (\J^-_1)^T\f^-_1 + (\M^-_1)^{-1}(\J^-_1)^T \frac{\partial \f^-_1}{\partial \m}
    \end{aligned}
    \right.
\end{equation}

Differentiate $[\q^-_1, \dq^-_1] = P(\q^+_0, \dq^+_0, \m, \tf, \dt_0)$:
\begin{align}
    &\left \{
    \begin{aligned}
    \frac{\partial \q^-_1}{\partial \q^+_0} =& \I  ,\; \frac{\partial \q^-_1}{\partial \dq^+_0} = \dt_0 \I \\
    \frac{\partial \q^-_1}{\partial \dt_0} =& \dq^+_0
    \end{aligned}
    \right. \\
    &\left \{
    \begin{aligned}
    \frac{\partial \dq^-_1}{\partial \q^+_0} =& \frac{\partial (\M^+_0)^{-1}}{\partial \q^+_0} (\dt_0(\tf - \corio^+_0) + (\J^+_0)^T\f^+_0) \\
    +& (\M^+_0)^{-1}(-\dt_0 \frac{\partial \corio^+_0}{\partial \q^+_0} + \frac{\partial (\J^+_0)^T}{\partial \q^+_0}\f^+_0) + (\J^+_0)^T\frac{\partial \f^+_0}{\partial \q^+_0}  \\
    \frac{\partial \dq^-_1}{\partial \dq^+_0} =& \I + (\M^+_0)^{-1}(-\dt_0 \frac{\partial \corio^+_0}{\partial \dq^+_0} + (\J^+_0)^T\frac{\partial \f^+_0}{\partial \dq^+_0}) \\
    \frac{\partial \dq^-_1}{\partial \tf} =& (\M^+_0)^{-1}(\dt_0 \I + (\J^+_0)^T \frac{\partial \f^+_0}{\partial \tf}) \\
    \frac{\partial \dq^-_1}{\partial \m} =& \frac{\partial (\M^+_0)^{-1}}{\partial \m} (\dt_0(\tf - \corio^+_0) + (\J^+_0)^T\f^+_0) \\ 
    +& (\M^+_0)^{-1}(-\dt_0 \frac{\partial \corio^+_0}{\partial \m} + (\J^+_0)^T \frac{\partial \f^+_0}{\partial \m}) \\
    \frac{\partial \dq^-_0}{\partial \dt_0} =& (\M^+_0)^{-1} ((\tf - \corio^+_0) + (\J^+_0)^T\f^+_0 / \dt_0)
    \end{aligned}
    \right.
\end{align}

Differentiate $\dt_0 = T(\q^+_0, \dq^+_0)$ and $\dt_1 = T(\q^+_1, \dq^+_1)$:
\begin{align}
    &\left \{
    \begin{aligned}
    \frac{\partial \dt_0}{\partial \q^+_0} =& \frac{(\J^+_0)_c}{(\J^+_0)_c \dq^+_0} ,\; \frac{\partial \dt_0}{\partial \dq^+_0} = \dt_0 \frac{(\J^+_0)_c}{(\J^+_0)_c \dq^+_0} \\
    \frac{\partial \dt_1}{\partial \q^+_1} =& \frac{(\J^+_1)_c}{(\J^+_1)_c \dq^+_1}  ,\; \frac{\partial \dt_1}{\partial \dq^+_1} = \dt_1 \frac{(\J^+_1)_c}{(\J^+_1)_c \dq^+_1} 
    \end{aligned}
    \right.
\end{align}

\newpage
